# Supplementary material for: Membrane mediated aggregation of curvature inducing nematogens and membrane tubulation
Source: arXiv:1302.1641 source file (2013-02-07)
Supplement: Supplementary file 1 [file Supplementary_Material.pdf]

## Persistence length of tubular membranes with nematic order

In this supplementary section we work out the free energy expression for a general fluid tubular membrane of uniform radius with nematic ordered membrane inclusions. The evaluation leads to an expression for persistence length of tubular membranes stabelized by nematicaly orderered membrane inclusions. The starting point for the evaluation is the general curvature free energy form for a fluid membrane equipped with nematic inclusions:

$$\mathscr{H}_{\text{anis}} = \oint dA \left\{ \frac{\kappa}{2}(2H)^2 + \frac{\kappa_\parallel}{2}(H_\parallel - H_\parallel^0)^2 + \frac{\kappa_\perp}{2}(H_\perp - H_\perp^0)^2 \right\} + \mathscr{H}_{\text{nem}}$$

The in-plane elastic free energy of the nematic ordering field has the form:

$$\mathscr{H}_{\text{nem}} = \frac{1}{2} K_A \oint dA \text{Tr} \left( \nabla \hat{m} : \nabla \hat{m} \right) \tag{1}$$

First, we consider a cylindrical membrane with nematic order free energy per tube length takes the simple form:

$$f := 2\pi r \left( \kappa_\parallel \left\{ \psi/r - H_\parallel^0 \right\}^2 + \kappa_\perp \left\{ (1-\psi)/r - H_\perp^0 \right\}^2 \right) + 2\kappa\pi/r \tag{2}$$

where $r$ is the tube radius, $\psi = \cos^2 \varphi$ is representing the orientation of the nematic field in the Darboux frame, which just follow the cylinder axis and the surface tangent perpendicular to it with principle curvatures 0 and $1/r$. The minimum free energy configuration obey the stationary condition, $\frac{\partial f}{\partial \psi} = 0$, $\frac{\partial f}{\partial r} = 0$ that gives,

$$\bar{r} = \sqrt{\frac{\left(\frac{\kappa}{2}\right)\left(\kappa_\parallel + \kappa_\perp\right) + \kappa_\perp \kappa_\parallel}{\kappa_\perp \kappa_\parallel \left(H_\parallel^0 + H_\perp^0\right)^2}} \tag{3}$$

and

$$\bar{\psi} = \cos^2 \bar{\varphi} = \frac{\left(\kappa_\parallel H_\parallel^0 - \kappa_\perp H_\perp^0\right)\bar{r} + \kappa_\perp}{\kappa_\perp + \kappa_\parallel}, \tag{4}$$

when $0 < \bar{\psi} < 1$, $\bar{\psi} = \frac{\kappa_\parallel H_\parallel^0 - \kappa_\perp H_\perp^0}{|H_\parallel^0 + H_\perp^0|(\kappa_\parallel + \kappa_\perp)} \sqrt{1 + \frac{\kappa}{2}\left(\frac{1}{\kappa_\parallel} + \frac{1}{\kappa_\perp}\right)} + \frac{\kappa_\perp}{\kappa_\parallel + \kappa_\perp}$. For parameters with $\bar{\psi} \leq 0$ the minimum free energy is obeys $\bar{\psi} = 0$ and $\bar{r} = \sqrt{\frac{\kappa_\perp + \kappa}{\kappa_\parallel (H_\parallel^0)^2 + \kappa_\perp (H_\perp^0)^2}}$ Similarly for $\bar{\psi} \geq 1$ the free energy minimum is found for $\bar{\psi} = 1$ and $\bar{r} = \sqrt{\frac{\kappa_\parallel + \kappa}{\kappa_\parallel (H_\parallel^0)^2 + \kappa_\perp (H_\perp^0)^2}}$. So, in general both $\bar{\varphi}$ and $\bar{r}$ are set by the model parameters. Eq. (1) is the only part of the free energy, which depends on the orientation of the nematogens. While the nematic elasticity gives a finite-size contribution for a cylinder with perfect nematic order, which will follow from the developments in the end of the Supplement. Nematic order means that the nematic

orientation will follow the geodesic lines on the cylinder. A well-known result from surface differential geometry that the geodesic lines on a cylinder in general are lines parallel to the long axis, circles perpendicular to the long axis or helical spirals, which are characterized by a fixed angle between the curve and the long axis of the helix (the first principal direction of the cylinder). The mean-field solution above precisely corresponds to that situation. In general, increasing $\kappa$ leads to increasing radius $\bar{r}$, while increasing $H_{\|}^0$ and $H_{\perp}^0$ leads to decreasing radius. Another important point is to ensure that the stationary solution found is a stable solution, i.e. the second derivative of $f$ is positive definite for the solution for $0 < \bar{\psi} < 1$.

$$\left(\begin{array}{cc} \frac{\partial^2 f}{\partial^2 \psi} & \frac{\partial^2 f}{\partial \psi \partial r} \\ \frac{\partial^2 f}{\partial r \partial \psi} & \frac{\partial^2 f}{\partial^2 r} \end{array}\right)_{\bar{\psi},\bar{r}} = \frac{2\pi}{\bar{r}^3} \left(\begin{array}{cc} (\kappa_{\|} + \kappa_{\perp})\bar{r}^2 & -(\kappa_{\|}\bar{\psi} - \kappa_{\perp} + \kappa_{\perp}\psi)\bar{r} \\ -(\kappa_{\|}\bar{\psi} - \kappa_{\perp} + \kappa_{\perp}\bar{\psi})\bar{r} & \kappa_{\|}\bar{\psi}^2 + \kappa_{\perp}(1-\bar{\psi})^2 + \frac{\kappa}{2} \end{array}\right) \tag{5}$$

Since the elastic moduli are all positive (or zero) this stability matrix positive definite for all parameter values with $\bar{r} > 0$. The stability matrix also gives us the possibility to evaluate the thermal fluctuations in a segment of the tubular membrane (over which the membrane can be considered as straight) in terms of these parameters. E.g. for a tube segment of length $\bar{r}$ we find:

$$\frac{\langle(\delta r)^2\rangle}{\bar{r}^2} = \frac{k_B T}{4\pi} \frac{\kappa_{\|} + \kappa_{\perp}}{\left\{\kappa_{\|}\kappa_{\perp} + (\kappa_{\|} + \kappa_{\perp})\frac{\kappa}{2}\right\}} \tag{6}$$

We note that if either $\kappa_{\|}$ or $\kappa_{\perp}$ is vanishing the variations in $r$ are inversly proportional to $\sqrt{\frac{\kappa}{k_B T}}$. So for a typical lipid membrane the ratio Eq.(6) is the order 0.001. If both $\kappa_{\perp}$ and $\kappa_{\|}$ the ratio is further reduced. For rigid membranes (with large $\kappa$) we can consider the thermally excited variations in $r$ for small. Similarly, we can estimate the thermal fluctuations in $x$ for such a segment:

$$\langle(\delta\psi)^2\rangle = \frac{k_B T}{4\pi} \frac{\kappa_{\|}\psi^2 + \kappa_{\|}(1-\psi)^2 + \frac{\kappa}{2}}{\left\{\kappa_{\|}\kappa_{\perp} + (\kappa_{\|} + \kappa_{\perp})\frac{\kappa}{2}\right\}} \tag{7}$$

which for rigid membranes become $\frac{1}{4\pi}\frac{k_B T}{\kappa_{\|}+\kappa_{\perp}}$. In the following we would like to investigate if the above observations can be generalized to include curved tubular surfaces as the results from computer simulations indicate. General tubular surfaces are also called canal surfaces and first we remind about some general nomenclature for curves and surfaces which is relevant for the analysis of canal surfaces.

# Space curves

First, let us consider a general curve $\mathcal{C}$ given vector representation $\vec{x}_C(t)$ in space, where $t$ represents a some parametrization of the curve. The length of the curve or the arc length is given by $s = \int_0^t |\vec{x}'_C(t')|^2 dt'$, which defines a very convenient parametrization of the curve (the natural representation). Derivatives with respect to $s$ are indicated by a dot. The vector $\vec{x}'_C(t)$ has the direction of the tangent of the curve. In the natural representation this vector is a unit tangent vector:

$$\vec{t} = \dot{\vec{x}}_C, \quad \vec{t}\vec{t} = 1 \Rightarrow \dot{\vec{t}}\vec{t} = 0 \tag{8}$$

It follows from Eq.(8) that $\dot{\vec{t}} \perp \vec{t}$ or $\vec{0}$. $\dot{\vec{t}}$ is thus in the normal plane of the curve $\vec{x_C}(s)$. The vector

$$\vec{p}(s) = \frac{\dot{\vec{t}}(s)}{|\dot{\vec{t}}(s)|} \tag{9}$$

is the unit normal principal normal vector to the curve at $\vec{x}(s)$. The normalization factor is called the local curvature $\lambda(s)$, its inverse is the curvature radius $r(s)$:

$$\lambda(s) = |\dot{\vec{t}}(s)| \tag{10}$$

$\vec{t}$ and $\vec{p}$ are perpendicular to each other and form together the *osculating* plane of the curve. To complete the frame we can introduce the binormal vector:

$$\vec{b}(s) = \vec{t}(s) \times \vec{p}(s) \tag{11}$$

The tuple $\vec{t}(s), \vec{p}(s), \vec{b}(s)$ form a so called moving frame of reference or the Frenet frame for the curve. Finaly, we introduce the torsion $\tau(s)$:

$$\tau(s) = -\vec{p}(s)\dot{\vec{b}}(s) \tag{12}$$

The quantities $\lambda(s)$ and $\tau(s)$ are invariant with respect change of parameters and completely fix the shape of the curve by the Frenet-Serret formula:

$$\begin{pmatrix} \dot{\vec{t}} \\ \dot{\vec{p}} \\ \dot{\vec{b}} \end{pmatrix} = \begin{pmatrix} 0 & \lambda(s) & 0 \\ -\lambda(s) & 0 & \tau(s) \\ 0 & -\tau(s) & 0 \end{pmatrix} \begin{pmatrix} \vec{t} \\ \vec{p} \\ \vec{b} \end{pmatrix} \tag{13}$$

# Canal surfaces

In the following we will introduce a class of surfaces, which is developed by circles of radius $r(s)$ with center $\vec{x}_C(s)$ and oriented in the normal plane of the curve. It is called a canal surface $\mathcal{S}$, with radius $r(s)$ and spine curve $\mathcal{C}$. The representation of a curve in the previous section makes the natural representation and the Frenet frame as a good starting point for the parameterization of the surface. The canal surface in terms of the spine curve $\mathcal{C}$ then has the form:

$$\vec{X}(s,\theta) = \vec{x}_c(s) + r(s)\left\{\cos\theta\,\vec{p}(s) + \sin\theta\,\vec{b}(s)\right\}. \tag{14}$$

The tangent vector along $s$ and $\theta$ then has the form,

$$\begin{aligned}
\partial_s\vec{X} &= [1-\lambda(s)r(s)\cos\theta]\,\vec{t}(s) + [\tau(s)r(s)\cos\theta + \dot{r}(s)\sin\theta]\,\vec{b}(s) \\
&\quad - [\tau(s)r(s)\sin\theta - \dot{r}(s)\cos\theta]\,\vec{p}(s) \\
\partial_\theta\vec{X} &= r(s)\cos\theta\,\vec{b}(s) - r(s)\sin\theta\,\vec{p}(s)
\end{aligned} \tag{15}$$

The basic intrinsic and extrinsic geometrical quantifiers can easily be established, for such canal surfaces.

Intrinsic geometry: We can now construct the metrical tensor of this class of canal surfaces:

$$\begin{aligned}
g_{\theta\theta} &= \partial_\theta\vec{X}\cdot\partial_\theta\vec{X} = r^2(s) \\
g_{\theta s} &= g_{s\theta} = \partial_\theta\vec{X}\cdot\partial_s\vec{X} = \tau(s)r^2(s) \\
g_{ss} &= \partial_s\vec{X}\cdot\partial_s\vec{X} = [1-\lambda(s)r(s)\cos\theta]^2 + [r(s)\tau(s)]^2 + \dot{r}^2(s)
\end{aligned} \tag{16}$$

The area element $dA = \sqrt{\det(g)}dsd\theta$ of the canal surface can thus be computed:

$$\sqrt{\det(g)} = \sqrt{[1-\lambda(s)r(s)\cos\theta]^2\,r^2(s) + r^2(s)\dot{r}^2(s)} \tag{17}$$

It can be noticed that the area element only depends on $\theta$ parameter. Also, we can calculate the inverse of the metric tensor:

$$[g]^{-1} = \frac{1}{\sqrt{\det(g)}}\begin{pmatrix} [1-\lambda(s)r(s)\cos\theta]^2 + [r(s)\tau(s)]^2 + \dot{r}^2(s) & -\tau(s)r^2(s) \\ -\tau(s)r^2(s) & r^2(s) \end{pmatrix}$$

which will be very useful in the construction of covariant vectors and tensors, Also, we are interested in the construction the differential operator. The Christoffel symbols $\Gamma_{\alpha\beta\gamma} = \frac{1}{2}\left(\partial_\alpha g_{\beta\gamma} + \partial_\beta g_{\gamma\alpha} - \partial_\gamma g_{\alpha\beta}\right)$ can now be computed since:

$$
\begin{aligned}
\partial_s g_{\theta\theta} &= 2r(s)\dot{r}(s), \quad \partial_s g_{s\theta} = \dot{\tau}(s)r^2(s) + 2\tau(s)r(s)\dot{r}(s) \\
\partial_s g_{ss} &= -2\cos\theta\left\{\dot{r}(s)\kappa(s) + r(s)\dot{\lambda}(s)\right\}\{1-\lambda(s)r(s)\cos\theta\} \\
&+ \ 2r(s)\tau(s)\{\dot{r}(s)\tau(s) + r(s)\dot{\tau}(s)\} + 2\dot{r}(s)\ddot{r}(s) \qquad (18) \\
\partial_\theta g_{ss} &= -2\lambda(s)r(s)\sin\theta\{1-\lambda(s)r(s)\cos\theta\} \\
\partial_\theta g_{s\theta} &= 0, \quad \partial_\theta g_{\theta\theta} = 0
\end{aligned}
$$

so,

$$
\begin{aligned}
\Gamma_{\theta\theta\theta} &= 0, \quad \Gamma_{s\theta\theta} = r(s)\dot{r}(s) \quad \Gamma_{\theta\theta s} = -r(s)\dot{r}(s), \quad \Gamma_{\theta s\theta} = r(s)\dot{r}(s) \\
\Gamma_{sss} &= -\cos\theta\left\{\dot{r}(s)\lambda(s) + r(s)\dot{\lambda}(s)\right\}\{1-\lambda(s)r(s)\cos\theta\} \\
&+ \ r(s)\tau(s)\{\dot{r}(s)\tau(s) + r(s)\dot{\tau}(s)\} + \dot{r}(s)\ddot{r}(s) \qquad (19) \\
\Gamma_{ss\theta} &= \lambda(s)r(s)\sin\theta\{1-\lambda(s)r(s)\cos\theta\} + \dot{\tau}(s)r^2(s) + 2\tau(s)r(s)\dot{r}(s), \\
\Gamma_{\theta ss} &= -\lambda(s)r(s)\sin\theta\{1-\lambda(s)r(s)\cos\theta\}, \qquad \Gamma_{s\theta s} = -\lambda(s)r(s)\sin\theta\{1-\lambda(s)r(s)\cos\theta\}
\end{aligned}
$$

Similarly we can calculate ${\Gamma_{\alpha\beta}}^{\gamma} = g^{\gamma\rho}\Gamma_{\alpha\beta\rho}$:

$$
\begin{aligned}
{\Gamma_{\theta\theta}}^{\theta} &= \frac{\tau(s)r^3(s)\dot{r}(s)}{r^2(s)\{1-\lambda(s)r(s)\cos\theta\}^2 + r^2(s)\dot{r}^2(s)} \\
{\Gamma_{\theta\theta}}^{s} &= -\frac{r(s)\dot{r}(s)}{\{1-\lambda(s)r(s)\cos\theta\}^2 + \dot{r}^2(s)}, \quad {\Gamma_{\theta s}}^{\theta} = -\frac{\tau(s)\lambda(s)r(s)\sin\theta}{1-\lambda(s)r(s)\cos\theta} \\
{\Gamma_{\theta\theta s}}^{s} &= \frac{\lambda(s)r(s)\sin\theta}{1-\lambda(s)r(s)\cos\theta}, \quad {\Gamma_{s\theta}}^{\theta} = -\frac{\tau(s)\lambda(s)r(s)\sin\theta}{1-\lambda(s)r(s)\cos\theta} \qquad (20) \\
{\Gamma_{\theta s}}^{s} &= \frac{\lambda(s)r(s)\sin\theta}{1-\lambda(s)r(s)\cos\theta}, \quad {\Gamma_{ss}}^{s} = \frac{\tau(s)\lambda(s)r(s)\sin\theta}{1-\lambda(s)r(s)\cos\theta} \\
{\Gamma_{ss}}^{\theta} &= \frac{\lambda}{r(s)}\frac{\sin\theta}{1-\lambda(s)r(s)\cos\theta}\left[\{1-\lambda(s)r(s)\cos\theta\}^2 + \{r(s)\tau(s)\}^2\right]
\end{aligned}
$$

With the Christoffel symbols can we analyse the canal surface for geodesics. For now we are just interested to know if the $s = const$ are geodesics, so vectors with a fixed angle with respect to that direction are parallel as assumed in Eq.(2) for the cylinder. The geodesic curvature for $s = const$ curves can be calculated from:

$$
\begin{aligned}
\kappa_g|_{s=const} &= -{\Gamma_{\theta\theta}}^{s}\sqrt{g}\, g_{ss}^{-\frac{3}{2}} \qquad (21) \\
&= \frac{-r(s)\dot{r}(s)}{\{1-\lambda(s)r(s)\cos\theta\}^2 + \dot{r}^2(s)} \frac{\sqrt{\{1-\lambda(s)r(s)\cos\theta\}^2 r^2(s) + \dot{r}^2(s)}}{\left[\{1-\lambda(s)r(s)\cos\theta\}^2 + \{r(s)\tau(s)\}^2 + \dot{r}^2(s)\right]^{3/2}}
\end{aligned}
$$

We notice that $s = const$ curves are not geodesic curves for a general canal surface. However, for canal surfaces where we can consider the radius as constant, this is indeed the case. We conclude that the geodesics form a constant angle with the $r = const.$ curves. For constant $r$ the ordered nematic field on the canal surface has a fixed angle with the meridian direction independent of $\lambda$ and $\tau$. We will later discus if this approximation is valid.

Extrinsic geometry: The extrinsic curvature properties depend on the second derivatives of $\vec{X}$:

$$\begin{aligned}
\partial_{ss}\vec{X} &= \left[r(s)\tau(s)\lambda(s)\sin\theta - \{\dot{r}(s)\tau(s) + r(s)\dot{\tau}(s)\}\cos\theta\right]\vec{t}(s) \\
&\quad + \left[\lambda(s) - \left\{\lambda^2(s) + \tau^2(s)\right\} r(s)\cos\theta - \{\tau(s)\dot{r}(s) + \dot{\tau}(s)r(s)\}\sin\theta\right]\vec{p}(s) \\
&\quad + \left[\{\dot{r}(s)\tau(s) + \dot{\tau}(s)r(s)\}\cos\theta - r(s)\tau^2(s)\sin\theta\right]\vec{b}(s) \\
\partial_{\theta\theta}\vec{X} &= -r(s)\cos\theta\,\vec{p}(s) - r(s)\sin\theta\,\vec{b}(s) \\
\partial_{s\theta}\vec{X} &= r(s)\lambda(s)\sin\theta\ \ \vec{t}(s) - \left[\tau(s)r(s)\cos\theta + \dot{r}(s)\right]\vec{p}(s) + \left[\dot{r}(s)\cos\theta - r(s)\tau(s)\sin\theta\right]\vec{b}(s)
\end{aligned} \tag{22}$$

The surface normal become:

$$\vec{N}(\theta, s) = -\sin\theta\,\vec{b}(s) - \cos\theta\,\vec{p}(s) \tag{23}$$

Similarly, the curvature tensor takes the form:

$$\begin{aligned}
K_{\theta\theta} &= \vec{N}(\theta, s)\cdot\partial_{\theta\theta}\vec{x} = r(s) \\
K_{s\theta} &= \vec{N}(\theta, s)\cdot\partial_{s\theta}\vec{x} = r(s)\tau(s) - \dot{r}(s)\cos\theta\sin\theta \\
K_{ss} &= \vec{N}(\theta, s)\cdot\partial_{ss}\vec{x} = -\lambda(s)\cos\theta + \tau^2(s)r(s) + \lambda^2(s)r(s)\cos^2\theta
\end{aligned} \tag{24}$$

and

$$\begin{aligned}
K^{\theta}_{\theta} &= \frac{1}{r(s)} + \frac{\tau(s)\dot{r}(s)\cos\theta\sin\theta}{\{1 - \lambda(s)r(s)\cos\theta\}^2 + \dot{r}^2(s)} \\
K^{\theta}_{s} &= \frac{r\tau\left\{1 - \lambda(s)r(s)\cos\theta + \dot{r}^2\right\} + \dot{r}(s)\cos\theta\sin\theta\left[r^2(s)\tau^2(s) - \{1 - \lambda(s)r(s)\cos\theta\}^2 + \dot{r}^2\right]}{r^2(s)\{1 - \lambda(s)r(s)\cos\theta\}^2 + r^2(s)\dot{r}^2(s)} \\
K^{s}_{\theta} &= \frac{-\dot{r}(s)\cos\theta\sin\theta}{\{1 - \lambda(s)r(s)\cos\theta\}^2 + \dot{r}^2(s)} \\
K^{s}_{s} &= \frac{-\lambda(s)\cos\theta + \lambda^2(s)r(s)\cos^2\theta + \tau\dot{r}\cos\theta\sin\theta}{\{1 - \lambda(s)r(s)\cos\theta\}^2 + \dot{r}^2(s)}
\end{aligned} \tag{25}$$

This is a fairly complex curvature matrix. However, it is simplified considerably in the limit where $r$ is constant (i.e. $\dot{r}(s) = 0$):

$$\{K^\alpha_\beta\} \to \begin{pmatrix} \frac{1}{r} & \frac{\tau(s)}{r\{1-\lambda(s)r\cos\theta\}} \\ & \\ 0 & \frac{-\lambda(s)\cos\theta}{1-\lambda(s)r\cos\theta} \end{pmatrix} \quad \text{for} \quad \dot{r}\to 0 \tag{26}$$

where $\alpha = \theta, s$ and $\beta = \theta, s$. The conformational variables $\lambda(s)$ and $\tau(s)$ of the canal surface are locally varying. In this limit we can quickly read off the principal curvatures:

$$c_1 = \frac{1}{r}, \qquad c_2(\theta, s) = \frac{-\lambda(s)\cos\theta}{1-\lambda(s)r\cos\theta} \tag{27}$$

where $c_2$ now depends on both $s$ and $\theta$, while $c_1$ is a constant. Notice that the dependence of the principal curvatures on $\dot{\kappa}$ and $\dot{\tau}$ also disappears with the $\dot{r} = 0$. The corresponding principal directions are:

$$\vec{e}_1(\theta, s) = \frac{\partial \vec{N}}{\partial\theta} = -\cos\theta\,\vec{b}(s) + \sin\theta\,\vec{p}(s), \qquad \vec{e}_2(\theta, s) = \vec{N}\times\vec{e}_1 = \vec{t}(s) \tag{28}$$

The mean curvature and the Gaussian curvature thus have the form:

$$\begin{aligned} H(\theta, s) &= \frac{1}{2}(c_1 + c_2(\theta, s)) = \frac{2\lambda(s)r\cos\theta - 1}{2r\{1-\lambda(s)r\cos\theta\}} \\ G(\theta, s) &= c_1 c_2(\theta, s) = \frac{-\lambda(s)\cos\theta}{r\{1-\lambda(s)r\cos\theta\}} \end{aligned} \tag{29}$$

where both $H$ and $G$ depends on $\theta$ and $s$. In the following, we will work in this constant $r$ limit. The physical significance of this approximation will be discussed in the end.

The curvature free energy: We are now in the position to calculate the free energy Eq.(1) of a helical canal surface. We will consider each contribution separately. First, the usual Helfrich term:

$$\begin{aligned} \mathscr{H}_{\text{sur}} = \frac{\kappa}{2}\int dA(2H)^2 &= \frac{\kappa}{2}\int_0^L ds \int_0^{2\pi} \frac{\{1-2r\lambda(s)\cos\theta\}^2}{1-\lambda(s)r\cos\theta} \\ &= \frac{\kappa}{2}\int_0^L ds\, d\theta\ \frac{1+4\lambda^2(s)r^2\cos^2\theta - 4\lambda(s)r\cos\theta}{r\{1-\lambda(s)r\cos\theta\}} \\ &= \frac{\kappa}{2r}\int_0^L ds \frac{2\pi}{\sqrt{1-(\lambda(s)r)^2}} \end{aligned} \tag{30}$$

The expression Eq.(31) is just the local version of the expression for Helfrich's curvature free energy for a constant $\lambda$ and $r$ canal surface. We will now continue with the terms involving

directional curvature elasticity.

Anisotropic elastic energy : Following Eq.(21) $s = const.$ curves are geodesics when $r$ is constant. Therefore we can consistently choose the directional curvature for a nematogen oriented with an angle $\varphi(s)$ with respect to the Darboux frame. With $\psi(s) = \cos^2(\varphi(s))$ and Eulers relations they become:

$$\begin{aligned} H_{\|}(\theta, s) &= \frac{\psi(s)}{r} - \frac{\lambda(s)\cos\theta}{1-\lambda(s)r\cos\theta}(1-\psi(s)), \\ H_{\perp}(\theta, s) &= \frac{1-\psi(s)}{r} - \frac{\lambda(s)\cos\theta}{1-\lambda(s)r\cos\theta}\psi(s), \end{aligned} \tag{31}$$

where $H_{\|}$ and $H_{\perp}$ both depends on $\theta$ and $s$. The remaining curvature elastic terms are:

$$\begin{aligned} \mathscr{H}_{\text{anis}}^{\|} &= \frac{\kappa_{\|}}{2}\int dA\left\{H_{\|}(\theta, s) - H_{\|}^{0}\right\}^2 \qquad (32) \\ &= \frac{\kappa_{\|}}{2}\int_0^L\int_0^{2\pi} r ds\, d\theta \frac{(1-\lambda(s)r\cos\theta)\left\{\left(\frac{\psi(s)}{r} - H_{\|}^{0}\right) + \left(H_{\|}^{0}\lambda(s)r - \lambda(s)\right)\cos\theta\right\}^2}{(1-\lambda(s)r\cos\theta)^2} \\ &= \frac{\kappa_{\|}}{2}\int_0^L ds\left\{r\frac{2\pi}{\sqrt{1-\lambda^2(s)r^2}}\left(\frac{1-\psi(s)}{r}\right)^2 + r2\pi\left(\frac{1}{r} - H_{\|}^{0}\right)\left(\frac{2\psi(s)-1}{r} - H_{\|}^{0}\right)\right\} \end{aligned}$$

and

$$\begin{aligned} \mathscr{H}_{\text{anis}}^{\perp} &= \frac{\kappa_{\perp}}{2}\int dA\left\{H_{\perp}(\theta, s) - H_{\perp}^{0}\right\}^2 \qquad (33) \\ &= \frac{\kappa_{\perp}}{2}\int_0^L\int_0^{2\pi} r ds\, d\theta\, \frac{\left\{\left[\frac{1}{r}(1-\psi(s)) - H_{\perp}^{0}\right] + \left[\kappa(s)rH_{\perp}^{0} - \lambda(s)\right]\cos\theta\right\}^2}{(1-\lambda(s)r\cos\theta)} \\ &= \frac{\kappa_{\perp}}{2}\int_0^L ds\left\{r\frac{2\pi}{\sqrt{1-(\lambda(s)r)^2}}\left(\frac{\psi(s)}{r}\right)^2 + r2\pi\left(\frac{1}{r} - H_{\perp}^{0}\right)\left(\frac{1-2\psi(s)}{r} - H_{\perp}^{0}\right)\right\} \end{aligned}$$

The nematic term:

Now, we can focus on the nematic term.

$$\mathscr{H}_{\text{nem}} = \frac{1}{2}\int_A K_1(Div(\hat{m}))^2 + K_3(Div(\hat{m}^{\perp}))^2 \tag{34}$$

Since we are only working in the one-constant approximation: $K_A = K_1 = K_3$, we can make use of the identity $(Div(\hat{m}))^2 + (Div(\hat{m}^{\perp}))^2 = (\mathrm{Tr}\,(\nabla\hat{m} : \nabla\hat{m}))^2 +$ total derivatives:

$$\mathcal{H}_{\rm nn} = \frac{1}{2}K_A\int d^2\xi\sqrt{g}{\rm Tr}\left(\nabla\hat{m}:\nabla\hat{m}\right) \tag{35}$$

$$= \frac{1}{2}K_A\int d^2\xi\sqrt{g}g^{\nu\mu}\left(\partial_\nu\hat{m}-\hat{N}(\hat{N}\partial_\nu\hat{m})\right)\left(\partial_\mu\hat{m}-\hat{N}(\hat{N}\partial_\mu\hat{m})\right)$$

$$= \frac{1}{2}K_A\int d^2\xi\sqrt{g}g^{\nu\mu}\left(\partial_\nu\varphi-A_\nu\right)\left(\partial_\mu\varphi-A_\mu\right) \tag{36}$$

$\hat{m}$ can here be chosen in any local orthonormal coordinate system:

$$\hat{m} = \cos\varphi\hat{e}_1+\sin\varphi\hat{e}_2 \tag{37}$$

It is a natural choice for us to use the principal directions for the curvature tensor: $\hat{e}_2=\hat{t}$ and $\hat{e}_1=\hat{e}_\theta$. We can now work out some of the ingredients in Eq(35). First we remember that

$$\hat{e}_1=\frac{\partial\hat{N}}{\partial\theta}=-\sin\theta\,\hat{p}+\cos\theta\,\hat{b},\qquad \hat{e}_2=\hat{t}. \tag{38}$$

The geometric vector potential $A_\nu=\hat{e}_1\partial_\nu\hat{e}_2$ takes in this basis the form:

$$A_\theta=\hat{e}_1\partial_\theta\hat{t}=0,\qquad A_s=\hat{e}_1\partial_s\hat{t}=-\lambda(s)\sin\theta. \tag{39}$$

Hence the self interaction of the nematic field can now be written as,

$$\begin{aligned}\mathscr{H}_{\rm nem} &= \frac{1}{2}K_A\int d\theta\,ds\frac{1}{r(1-\lambda(s)r\cos\theta)} \\ &\quad \left\{\left[(1-\lambda(s)r\cos\theta)^2+r^2\tau^2(s)\right](\partial_\theta\varphi)^2+r^2\left[\partial_s\varphi+\lambda(s)\sin\theta\right]^2\right. \\ &\quad \left.-2\tau(s)r^2\partial_s\varphi\,\partial_\theta\varphi-2\tau(s)r^2\lambda(s)\sin\theta\partial_\theta\varphi\right\}.\end{aligned} \tag{40}$$

For the ansatz $\varphi(s)=\varphi_0$, the free energy become:

$$\mathscr{H}_{\rm nem} = \frac{K_A}{2}\int_0^L ds\frac{2\pi r}{\sqrt{1-(\lambda(s)r)^2}}\left(\lambda(s)^2-\lambda(s)^2\frac{1-\sqrt{1-(\lambda(s)r)^2}}{(\lambda(s)r)^2}\right)$$

$$= \frac{K_A}{2}\frac{2\pi}{r}\int_0^L ds\left(1-\sqrt{1-(\lambda(s)r)^2}\right). \tag{41}$$

We can put together the elastic free energy from the curvature contributions and the nematic contributions to the free energy.

$$\mathscr{H}_{\rm tot} = \mathscr{H}_{\rm nem}+\mathscr{H}_{\rm sur}+\mathscr{H}^{\parallel}_{\rm anis}+\mathscr{H}^{\perp}_{\rm anis} \tag{42}$$

$$= \frac{2\pi}{r}\frac{K_A}{2}\int_0^L ds\left\{1-\sqrt{1-\lambda^2(s)r^2}\right\}+\frac{2\pi}{r}\int_0^L ds\left\{\frac{\frac{\kappa}{2}+\frac{\kappa_\parallel}{2}(1-\psi(s))^2+\frac{\kappa_\perp}{2}\psi(s)^2}{\sqrt{1-\lambda^2(s)r^2}}\right\}$$

$$+ \int_0^L ds\frac{2\pi}{r}\left\{\frac{\kappa_\parallel}{2}(1-rH^0_\parallel)\left[2\psi(s)-1-rH^0_\parallel\right]+\frac{\kappa_\perp}{2}(1-rH^0_\perp)\left[1-2\psi(s)-rH^0_\perp\right]\right\}$$

A simple stability analysis of the total free energy show that the elastic free energies actually are minimal for $\kappa = 0$, which corresponds to the cylinder solution discussed in the beginning. The stability matrix Eq.(5) is thus extended with one positive diagonal term:

$$
\begin{pmatrix}
\frac{\partial^2 f_{\text{tot}}}{\partial^2\psi} & \frac{\partial^2 f_{\text{tot}}}{\partial\psi\partial r} & \frac{\partial^2 f_{\text{tot}}}{\partial\psi\partial\lambda} \\
\frac{\partial^2 f_{\text{tot}}}{\partial r\partial\psi} & \frac{\partial^2 f_{\text{tot}}}{\partial r^2} & \frac{\partial^2 f_{\text{tot}}}{\partial r\partial\lambda} \\
\frac{\partial^2 f_{\text{tot}}}{\partial\lambda\partial\psi} & \frac{\partial^2 f_{\text{tot}}}{\partial\lambda\partial r} & \frac{\partial^2 f_{\text{tot}}}{\partial\lambda^2}
\end{pmatrix}_{\bar\psi,\bar r,\kappa=0} = \tag{43}
$$

$$
\frac{4\pi}{\bar r^3}\begin{pmatrix}
(\kappa_\| + \kappa_\perp)\bar r^2 & -(\kappa_\|\bar\psi - \kappa_\perp + \kappa_\perp\psi)\bar r & 0 \\
-(\kappa_\|\bar\psi - \kappa_\perp + \kappa_\perp\bar\psi)\bar r & \kappa_\|\bar\psi^2 + \kappa_\perp(1-\bar\psi)^2 + \frac{\kappa}{2} & 0 \\
0 & 0 & \left(K_A + \kappa + \kappa_\|(1-\bar\psi)^2 + \kappa_\perp\bar\psi^2\right)\frac{\bar r^4}{4}
\end{pmatrix}
$$

Thus for configurations with small spine line curvatures $\lambda$ we observe that the coupling between $\lambda$ and the variables $r$ and $\psi$ are vanishing. We can therefore approximatively write the free energy of deviations away from the tube configuration:

$$
\Delta F_{\text{tot}} \approx \frac{1}{2}\pi\bar r\left(K_A + \kappa + \kappa_\|(1-\bar\psi)^2 + \kappa_\perp\bar\psi^2\right)\int_0^L ds\lambda^2(s) \tag{44}
$$

The corresponding persistence length:

$$
l_P = \frac{\pi\bar r\left(K_A + \kappa + \kappa_\|(1-\bar\psi)^2 + \kappa_\perp\bar\psi^2\right)}{k_B T} \tag{45}
$$

# Curvature mediated aggregation

In this section we demonstrate the importance of the protein induced deformation (spontaneous curvature) in aggregation of the nematogens. Fig. 1 shows the pattern of nematogen aggregation and orientation on an infinitely rigid membrane ($\kappa = \infty$) with $C_0^\| = 0.5$ and $\epsilon_{LL} = 3$. In the absence of the explicit membrane nematic interaction, by setting $\kappa_\| = 0$, we observe that the nematogens do not orient and remain in an isotropic phase, as in Fig. 1(a) and (b). Further, we also do not observe aggregation of nematogens. In the infinite limit, when the nematic membrane interactions exists, as in Fig. 1 (c) where $\kappa_\| = 10$, the nematogens tends to orient and aggregate. The order and aggregation becomes more pronounced when the membrane becomes soft, characteristic of a biological membrane with $\kappa = 10 - 100 k_B T$.

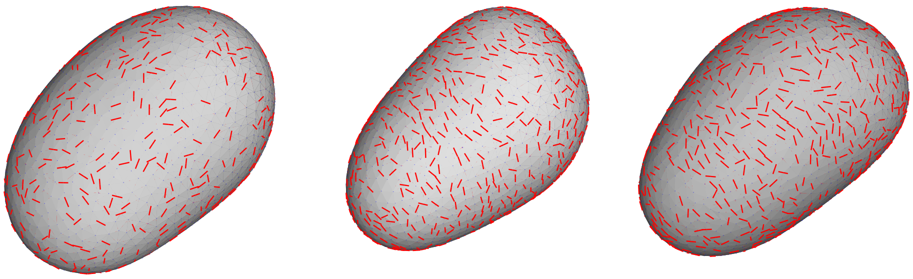

a) $\kappa_{\parallel} = 0$, $\phi_A = 0.3$ b) $\kappa_{\parallel} = 0$, $\phi_A = 0.5$ c) $\kappa_{\parallel} = 10$, $\phi_A = 0.5$

Figure 1: Aggregation of curvature inducing nematogens on a membrane with $\kappa = \infty$, $C_0^{\parallel} = 0.5$ and $\epsilon_{LL} = 3k_BT$. Nematogens in the isotropic phase when the curvature induced deformations are nullified by setting $\kappa_{\parallel} = 0$, $\phi_A = 0.3$(a) and $\phi_A = 0.5$(b). The nematogens starts to aggregate and orient when the nematic-membrane interaction is switched on by setting $\kappa_{\parallel} = 10$, as shown in (c).
